# Supplementary material for: Supersaliency: A Novel Pipeline for Predicting Smooth Pursuit-Based Attention Improves Generalizability of Video Saliency
Source: arXiv:1801.08925 ancillary file (2019-04-12)
Supplement: Supplementary file 1 [file supplementaryMaterial.pdf]

# Supplementary Material for:
# Supersaliency: A Novel Pipeline for Predicting Smooth Pursuit-Based Attention Improves Generalizability of Video Saliency

Mikhail Startsev, Michael Dorr
Technical University of Munich
{mikhail.startsev, michael.dorr}@tum.de

## Abstract

*The tables below represent full evaluation results on all data sets: Results with individual metrics' average values for GazeCom [1] are presented in Tables 1 to 3 ("SP" – smooth pursuit, "FIX" – fixation, and "onset" conditions, respectively), for a subset of 50 Hollywood2 [2] test clips – in Tables 4 to 6 ("SP", "FIX", and "onset" conditions, respectively), for CITIUS-R [3] – in Table 7 ("onset" condition).*

## References

[1] M. Dorr, T. Martinetz, K. R. Gegenfurtner, and E. Barth, "Variability of eye movements when viewing dynamic natural scenes," *Journal of Vision*, vol. 10, no. 10, p. 28, 2010. [Online]. Available: +http://dx.doi.org/10.1167/10.10.28

[2] S. Mathe and C. Sminchisescu, "Dynamic eye movement datasets and learnt saliency models for visual action recognition," in *Proceedings of the 12th European Conference on Computer Vision - Volume Part II*, ser. ECCV'12. Berlin, Heidelberg: Springer-Verlag, 2012, pp. 842–856. [Online]. Available: http://dx.doi.org/10.1007/978-3-642-33709-3_60

[3] V. Leborán, A. García-Díaz, X. R. Fdez-Vidal, and X. M. Pardo, "Dynamic whitening saliency," *IEEE Transactions on Pattern Analysis and Machine Intelligence*, vol. 39, no. 5, pp. 893–907, May 2017.

[4] M. Startsev, I. Agtzidis, and M. Dorr, "Smooth pursuit," http://michaeldorr.de/smoothpursuit/, 2016.

[5] T. Judd, F. Durand, and A. Torralba, "A benchmark of computational models of saliency to predict human fixations," http://hdl.handle.net/1721.1/68590, 2012.

Table 1. Supersaliency (SP) prediction results on GazeCom (manually annotated SP samples). Weighted averaging was used in all columns marked with *, but average ranks (i.e. the averages of the ranks for all 9 metrics) are provided both for weighted and regular averaging of statistics. The rows are sorted by the mean rank for the weighted averaging column. xAUC was not considered for mean ranks computation. Top-3 non-baseline results in each column are **boldified**.

| Model | AUC-Borji* | AUC-Judd* | sAUC* | accuracy* | NSS* | SIM* | CC* | KLD* | IG* | avg. rank | avg. rank* | xAUC* |
|---|---|---|---|---|---|---|---|---|---|---|---|---|
| Infinite Humans | 1.00 | 0.99 | 1.00 | 1.00 | 31.38 | 1.00 | 1.00 | 0.00 | 11.30 | 2.67 | 1.00 | 0.97 |
| *S-CNN SP* | **0.84** | **0.93** | **0.79** | **0.78** | **1.65** | 0.18 | **0.25** | **2.45** | **3.36** | 10.89 | **3.00** | 0.59 |
| *S-CNN SP + Gravity CB* | **0.83** | 0.92 | 0.76 | **0.78** | **1.53** | 0.18 | **0.23** | **2.47** | **3.31** | 15.78 | **4.89** | 0.54 |
| *S-CNN FIX* | 0.81 | 0.92 | 0.76 | 0.76 | 1.43 | 0.16 | 0.20 | **2.55** | 3.20 | 19.44 | **9.11** | 0.54 |
| GBVS | 0.80 | 0.92 | 0.69 | 0.73 | 1.46 | 0.17 | 0.20 | 2.59 | **3.25** | 17.78 | 11.11 | 0.58 |
| Invariant-K | 0.80 | 0.92 | 0.78 | 0.75 | 1.53 | **0.20** | **0.21** | 5.89 | 0.25 | 12.78 | 11.33 | 0.62 |
| PMES | 0.82 | 0.92 | **0.80** | **0.77** | 1.39 | 0.18 | 0.19 | 5.76 | 1.09 | 10.22 | 11.78 | **0.71** |
| *S-CNN FIX + Gravity CB* | 0.81 | 0.91 | 0.73 | 0.75 | 1.33 | 0.16 | 0.19 | 2.56 | 3.18 | 20.89 | 12.22 | 0.50 |
| MCSDM | **0.82** | 0.91 | **0.80** | 0.76 | 1.29 | 0.17 | 0.16 | 4.51 | 2.20 | 19.22 | 13.44 | **0.71** |
| PIM-ZEN | 0.80 | 0.92 | 0.78 | 0.75 | 1.46 | 0.16 | 0.17 | 5.33 | 1.73 | 15.67 | 13.56 | 0.69 |
| OBDL-T | 0.79 | 0.91 | 0.76 | 0.74 | 1.31 | 0.16 | 0.17 | 3.06 | 3.10 | **5.89** | 13.67 | 0.63 |
| OBDL-MRF-O | 0.79 | 0.91 | 0.76 | 0.74 | 1.27 | 0.17 | 0.17 | 3.10 | 3.04 | **5.33** | 13.78 | 0.62 |
| PNSP-CS | 0.78 | **0.92** | 0.75 | 0.71 | 1.51 | 0.17 | 0.18 | 2.96 | 2.89 | 19.78 | 13.89 | 0.71 |
| PIM-MCS | 0.80 | 0.92 | 0.78 | 0.74 | 1.41 | 0.16 | 0.16 | 5.18 | 1.88 | 16.11 | 14.33 | 0.68 |
| OBDL-S | 0.79 | 0.91 | 0.76 | 0.74 | 1.31 | 0.16 | 0.17 | 3.19 | 3.06 | 8.33 | 14.67 | 0.63 |
| AWS-D | 0.79 | 0.91 | 0.77 | 0.73 | 1.29 | 0.15 | 0.17 | 2.67 | 3.09 | 15.22 | 14.89 | 0.57 |
| OBDL-MRF-OC | 0.79 | 0.91 | 0.76 | 0.74 | 1.26 | 0.17 | 0.17 | 3.10 | 3.03 | **7.11** | 15.11 | 0.62 |
| OBDL-MRF-C | 0.79 | 0.91 | 0.76 | 0.74 | 1.25 | 0.16 | 0.17 | 3.10 | 3.02 | 8.67 | 16.33 | 0.62 |
| MSM-SM | 0.77 | **0.93** | 0.75 | 0.73 | **1.65** | **0.19** | 0.19 | 10.43 | -4.26 | 19.22 | 16.78 | **0.74** |
| STSD | 0.78 | 0.91 | 0.77 | 0.73 | 1.17 | 0.16 | 0.15 | 2.98 | 2.96 | 22.11 | 18.00 | 0.64 |
| OBDL-MRF-TO | 0.78 | 0.91 | 0.75 | 0.73 | 1.17 | 0.16 | 0.16 | 3.08 | 2.97 | 11.44 | 18.56 | 0.60 |
| One Human | 0.69 | 0.93 | 0.69 | 0.64 | 2.60 | 0.20 | 0.31 | 12.67 | -11.01 | 20.11 | 18.67 | 0.67 |
| OBDL-MRF | 0.78 | 0.91 | 0.75 | 0.73 | 1.18 | 0.16 | 0.16 | 3.10 | 2.97 | 12.00 | 18.89 | 0.61 |
| OBDL-MRF-TC | 0.78 | 0.91 | 0.75 | 0.73 | 1.16 | 0.16 | 0.16 | 3.08 | 2.96 | 13.56 | 20.56 | 0.60 |
| OBDL | 0.78 | 0.91 | 0.76 | 0.73 | 1.23 | 0.15 | 0.14 | 4.76 | 2.19 | 17.89 | 22.44 | 0.63 |
| OBDL-MRF-T | 0.78 | 0.91 | 0.74 | 0.73 | 1.13 | 0.16 | 0.16 | 3.11 | 2.92 | 15.56 | 23.11 | 0.59 |
| ACLNet | 0.77 | 0.91 | 0.66 | 0.71 | 0.98 | **0.18** | 0.15 | 4.02 | 1.51 | 24.89 | 24.33 | 0.45 |
| DeepVS (OMCNN-2CLSTM) | 0.74 | 0.91 | 0.65 | 0.68 | 1.09 | 0.16 | 0.16 | 3.48 | 2.05 | 26.44 | 25.44 | 0.48 |
| MAM | 0.72 | 0.91 | 0.71 | 0.67 | 1.12 | 0.15 | 0.14 | 9.55 | -4.42 | 27.67 | 27.89 | 0.66 |
| Invariant-S | 0.72 | 0.91 | 0.70 | 0.69 | 0.98 | 0.15 | 0.13 | 6.27 | -0.87 | 28.44 | 28.56 | 0.54 |
| Centre | 0.67 | 0.90 | 0.50 | 0.62 | 0.59 | 0.15 | 0.10 | 3.21 | 2.06 | 29.56 | 29.44 | 0.44 |
| Invariant-H | 0.71 | 0.90 | 0.69 | 0.68 | 0.94 | 0.15 | 0.13 | 6.22 | -0.90 | 29.89 | 29.78 | 0.55 |
| Chance | 0.50 | 0.89 | 0.50 | 0.50 | 0.00 | 0.10 | -0.00 | 3.35 | 1.83 | 31.11 | 31.00 | 0.50 |
| Permutation | 0.53 | 0.89 | 0.50 | 0.52 | 0.01 | 0.04 | 0.00 | 15.33 | -15.24 | 33.33 | 33.44 | 0.48 |

Table 2. Saliency (fixations) prediction results on GazeCom (manually annotated fixation samples). Regular averaging was used in all columns with individual metrics, but mean ranks are provided for weighted averaging of statistics as well (marked with $^*$). The rows are sorted by the mean rank for the regular averaging column. Top-3 non-baseline results in each column are **boldified**.

| Model | AUC-Borji | AUC-Judd | sAUC | accuracy | NSS | SIM | CC | KLD | IG | avg. rank | avg. rank$^*$ |
|---|---|---|---|---|---|---|---|---|---|---|---|
| Infinite Humans | 0.88 | 1.00 | 0.82 | 0.79 | 5.45 | 1.00 | 1.00 | 0.00 | 3.08 | 1.00 | 1.00 |
| *S-CNN FIX + Gravity CB* | **0.80** | **0.92** | 0.69 | **0.74** | **1.34** | **0.45** | **0.47** | **1.02** | **0.58** | **2.78** | **2.78** |
| *S-CNN SP + Gravity CB* | **0.79** | **0.92** | 0.68 | **0.73** | **1.36** | **0.46** | **0.47** | **1.06** | **0.52** | **2.89** | **2.89** |
| *S-CNN SP* | 0.78 | **0.91** | **0.70** | **0.72** | **1.28** | 0.44 | **0.44** | 1.11 | 0.46 | **4.44** | **4.33** |
| *S-CNN FIX* | **0.78** | 0.91 | **0.72** | 0.72 | 1.24 | 0.43 | 0.42 | **1.08** | **0.50** | 4.56 | 4.56 |
| AWS-D | 0.74 | 0.91 | **0.69** | 0.68 | 1.05 | 0.41 | 0.36 | 1.20 | 0.33 | 7.89 | 8.22 |
| DeepVS (OMCNN-2CLSTM) | 0.75 | 0.91 | 0.62 | 0.69 | 1.04 | 0.42 | 0.35 | 1.51 | -0.06 | 9.78 | 9.22 |
| ACLNet | 0.77 | 0.91 | 0.62 | 0.72 | 1.21 | **0.44** | 0.42 | 2.37 | -1.27 | 11.00 | 10.22 |
| GBVS | 0.74 | 0.91 | 0.61 | 0.69 | 1.02 | 0.42 | 0.35 | 1.23 | 0.27 | 11.22 | 11.33 |
| OBDL-MRF-O | 0.71 | 0.91 | 0.66 | 0.67 | 0.98 | 0.39 | 0.33 | 2.37 | -1.26 | 12.22 | 12.56 |
| OBDL-MRF-TC | 0.71 | 0.91 | 0.66 | 0.67 | 0.98 | 0.39 | 0.33 | 2.32 | -1.21 | 12.89 | 13.11 |
| OBDL-MRF-T | 0.71 | 0.91 | 0.65 | 0.66 | 0.99 | 0.39 | 0.33 | 2.29 | -1.17 | 13.22 | 13.22 |
| OBDL-MRF-OC | 0.71 | 0.91 | 0.66 | 0.67 | 0.97 | 0.38 | 0.33 | 2.37 | -1.26 | 13.89 | 14.33 |
| OBDL-MRF-TO | 0.71 | 0.91 | 0.66 | 0.67 | 0.98 | 0.39 | 0.33 | 2.33 | -1.22 | 13.89 | 14.22 |
| OBDL-T | 0.71 | 0.91 | 0.66 | 0.66 | 0.97 | 0.38 | 0.32 | 2.29 | -1.16 | 15.11 | 15.44 |
| OBDL-MRF | 0.71 | 0.91 | 0.66 | 0.67 | 0.96 | 0.38 | 0.32 | 2.35 | -1.25 | 16.00 | 16.44 |
| OBDL-MRF-C | 0.71 | 0.91 | 0.66 | 0.67 | 0.96 | 0.38 | 0.32 | 2.37 | -1.26 | 16.11 | 16.56 |
| Centre | 0.71 | 0.90 | 0.50 | 0.66 | 0.84 | 0.40 | 0.32 | 1.47 | -0.13 | 16.78 | 15.67 |
| One Human | 0.71 | 0.92 | 0.66 | 0.66 | 1.06 | 0.21 | 0.29 | 9.73 | -11.59 | 19.22 | 19.22 |
| OBDL-S | 0.70 | 0.91 | 0.65 | 0.66 | 0.94 | 0.38 | 0.31 | 2.74 | -1.79 | 19.78 | 19.89 |
| Invariant-K | 0.70 | 0.91 | 0.66 | 0.66 | 0.91 | 0.35 | 0.29 | 5.91 | -5.55 | 20.78 | 20.56 |
| STSD | 0.67 | 0.90 | 0.65 | 0.64 | 0.54 | 0.32 | 0.16 | 1.81 | -0.48 | 21.56 | 21.67 |
| Invariant-S | 0.69 | 0.90 | 0.66 | 0.66 | 0.75 | 0.35 | 0.23 | 4.84 | -4.22 | 21.89 | 21.22 |
| OBDL | 0.67 | 0.90 | 0.64 | 0.63 | 0.82 | 0.33 | 0.26 | 4.77 | -4.33 | 23.22 | 23.33 |
| Invariant-H | 0.67 | 0.90 | 0.64 | 0.64 | 0.64 | 0.34 | 0.20 | 4.77 | -4.15 | 23.67 | 23.56 |
| PIM-MCS | 0.65 | 0.90 | 0.62 | 0.62 | 0.61 | 0.31 | 0.19 | 5.54 | -5.41 | 25.89 | 26.00 |
| PIM-ZEN | 0.65 | 0.90 | 0.62 | 0.62 | 0.64 | 0.30 | 0.20 | 5.67 | -5.59 | 26.44 | 26.44 |
| PMES | 0.64 | 0.90 | 0.61 | 0.61 | 0.62 | 0.29 | 0.20 | 6.50 | -6.81 | 27.78 | 27.78 |
| Chance | 0.50 | 0.89 | 0.50 | 0.50 | -0.00 | 0.30 | -0.00 | 1.85 | -0.71 | 28.00 | 28.00 |
| MCSDM | 0.64 | 0.90 | 0.60 | 0.61 | 0.44 | 0.29 | 0.14 | 5.45 | -5.49 | 28.44 | 28.67 |
| PNSP-CS | 0.61 | 0.89 | 0.57 | 0.58 | 0.32 | 0.28 | 0.10 | 2.47 | -1.51 | 28.67 | 28.89 |
| Permutation | 0.63 | 0.89 | 0.50 | 0.59 | 0.35 | 0.26 | 0.13 | 4.48 | -4.40 | 29.33 | 29.00 |
| MAM | 0.58 | 0.89 | 0.56 | 0.56 | 0.33 | 0.22 | 0.10 | 10.49 | -12.48 | 31.56 | 31.67 |
| MSM-SM | 0.54 | 0.89 | 0.53 | 0.52 | 0.30 | 0.12 | 0.10 | 15.09 | -19.37 | 33.11 | 33.00 |

Table 3. Saliency (fixation onsets, detection as in [1]) prediction results on GazeCom. Regular averaging was used in all columns with individual metrics, but mean ranks are provided for weighted averaging of statistics as well (marked with *). The rows are sorted by the mean rank for the regular averaging column. Top-3 non-baseline results in each column are **boldified**.

| Model | AUC-Borji | AUC-Judd | sAUC | accuracy | NSS | SIM | CC | KLD | IG | avg. rank | avg. rank* |
|---|---|---|---|---|---|---|---|---|---|---|---|
| Infinite Humans | 0.87 | 1.00 | 0.79 | 0.78 | 5.34 | 1.00 | 1.00 | 0.00 | 3.34 | 1.00 | 1.00 |
| *S-CNN FIX + Gravity CB* | **0.79** | **0.92** | 0.69 | **0.73** | **1.31** | **0.46** | **0.48** | **0.98** | **0.52** | **2.78** | **2.78** |
| *S-CNN SP + Gravity CB* | **0.78** | **0.92** | 0.68 | **0.73** | **1.33** | **0.47** | **0.49** | **1.03** | **0.46** | **2.89** | **2.89** |
| *S-CNN SP* | **0.78** | **0.91** | **0.70** | **0.72** | **1.26** | **0.45** | **0.46** | 1.07 | 0.41 | **4.11** | **4.11** |
| *S-CNN FIX* | 0.77 | 0.91 | **0.71** | 0.72 | 1.21 | 0.44 | 0.43 | **1.04** | **0.45** | 4.78 | 4.78 |
| AWS-D | 0.74 | 0.91 | **0.69** | 0.68 | 1.04 | 0.42 | 0.37 | 1.16 | 0.29 | 7.44 | 7.56 |
| GBVS | 0.75 | 0.91 | 0.61 | 0.69 | 1.04 | 0.43 | 0.37 | 1.17 | 0.26 | 10.11 | 9.78 |
| ACLNet | 0.77 | 0.91 | 0.62 | 0.71 | 1.18 | 0.45 | 0.43 | 2.37 | -1.34 | 10.67 | 10.78 |
| DeepVS (OMCNN-2CLSTM) | 0.74 | 0.91 | 0.61 | 0.68 | 0.99 | 0.42 | 0.36 | 1.52 | -0.19 | 11.00 | 10.44 |
| OBDL-MRF-O | 0.71 | 0.91 | 0.66 | 0.67 | 0.96 | 0.39 | 0.34 | 2.37 | -1.29 | 11.89 | 12.44 |
| OBDL-T | 0.71 | 0.91 | 0.66 | 0.67 | 0.96 | 0.39 | 0.33 | 2.28 | -1.18 | 12.44 | 12.44 |
| OBDL-MRF-OC | 0.71 | 0.91 | 0.66 | 0.67 | 0.95 | 0.39 | 0.33 | 2.37 | -1.30 | 13.67 | 14.44 |
| OBDL-MRF-TC | 0.71 | 0.91 | 0.66 | 0.67 | 0.94 | 0.39 | 0.33 | 2.32 | -1.26 | 14.22 | 14.67 |
| OBDL-MRF-TO | 0.71 | 0.91 | 0.66 | 0.66 | 0.94 | 0.39 | 0.33 | 2.33 | -1.27 | 14.78 | 15.44 |
| OBDL-MRF-T | 0.71 | 0.91 | 0.65 | 0.66 | 0.94 | 0.39 | 0.34 | 2.30 | -1.22 | 14.89 | 15.44 |
| OBDL-MRF-C | 0.71 | 0.91 | 0.66 | 0.67 | 0.94 | 0.39 | 0.33 | 2.37 | -1.30 | 16.00 | 16.22 |
| OBDL-MRF | 0.71 | 0.91 | 0.66 | 0.67 | 0.93 | 0.39 | 0.33 | 2.35 | -1.29 | 16.33 | 16.56 |
| Centre | 0.71 | 0.90 | 0.50 | 0.66 | 0.82 | 0.41 | 0.33 | 1.43 | -0.18 | 16.44 | 15.67 |
| OBDL-S | 0.70 | 0.91 | 0.65 | 0.66 | 0.94 | 0.39 | 0.32 | 2.74 | -1.78 | 18.44 | 18.78 |
| Invariant-K | 0.70 | 0.91 | 0.66 | 0.65 | 0.93 | 0.37 | 0.30 | 5.97 | -5.76 | 19.56 | 18.67 |
| STSD | 0.67 | 0.90 | 0.65 | 0.64 | 0.55 | 0.33 | 0.17 | 1.75 | -0.50 | 21.56 | 21.56 |
| Invariant-S | 0.68 | 0.90 | 0.65 | 0.65 | 0.74 | 0.36 | 0.24 | 4.97 | -4.53 | 22.22 | 21.78 |
| OBDL | 0.67 | 0.90 | 0.64 | 0.64 | 0.82 | 0.34 | 0.26 | 4.76 | -4.27 | 22.44 | 22.56 |
| One Human | 0.69 | 0.91 | 0.64 | 0.64 | 0.94 | 0.21 | 0.28 | 10.25 | -12.43 | 22.56 | 22.33 |
| Invariant-H | 0.67 | 0.90 | 0.64 | 0.64 | 0.64 | 0.35 | 0.21 | 4.90 | -4.48 | 24.44 | 24.11 |
| PIM-MCS | 0.65 | 0.90 | 0.63 | 0.62 | 0.62 | 0.31 | 0.21 | 5.51 | -5.64 | 26.11 | 26.11 |
| PIM-ZEN | 0.65 | 0.90 | 0.62 | 0.61 | 0.65 | 0.31 | 0.22 | 5.63 | -5.82 | 26.33 | 26.44 |
| PMES | 0.65 | 0.90 | 0.62 | 0.61 | 0.66 | 0.30 | 0.22 | 6.39 | -6.85 | 27.00 | 27.00 |
| Chance | 0.50 | 0.89 | 0.50 | 0.50 | 0.00 | 0.30 | -0.00 | 1.79 | -0.74 | 28.00 | 28.00 |
| MCSDM | 0.64 | 0.90 | 0.62 | 0.61 | 0.47 | 0.30 | 0.16 | 5.38 | -5.59 | 28.33 | 28.56 |
| PNSP-CS | 0.61 | 0.89 | 0.58 | 0.58 | 0.37 | 0.30 | 0.12 | 2.38 | -1.80 | 28.67 | 28.00 |
| Permutation | 0.63 | 0.89 | 0.51 | 0.59 | 0.41 | 0.27 | 0.16 | 4.52 | -4.56 | 29.44 | 29.22 |
| MAM | 0.58 | 0.89 | 0.57 | 0.56 | 0.36 | 0.23 | 0.12 | 10.25 | -12.38 | 32.11 | 32.11 |
| MSM-SM | 0.55 | 0.90 | 0.54 | 0.53 | 0.38 | 0.14 | 0.12 | 14.56 | -18.53 | 32.33 | 32.33 |

Table 4. Supersaliency (SP) prediction results on Hollywood2, 50-clip subset (SP samples detected by [4]). Weighted averaging was used in all columns marked with *, but average ranks (i.e. the averages of the ranks for all 9 metrics) are provided both for weighted and regular averaging of statistics. The rows are sorted by the mean rank for the weighted averaging column. xAUC was not considered for mean ranks computation. Top-3 non-baseline results in each column are **boldified**. In the *Infinite Humans* row, the "inf" value indicates that the sequence, which is analysed in order to get the estimate for this baseline [5], does not seem to converge, at least on the available data.

| Model | AUC-Borji* | AUC-Judd* | sAUC* | accuracy* | NSS* | SIM* | CC* | KLD* | IG* | avg. rank | avg. rank* | xAUC* |
|---|---|---|---|---|---|---|---|---|---|---|---|---|
| Infinite Humans | 1.00 | 0.99 | 1.00 | 0.94 | inf | 1.00 | 1.00 | 0.00 | 5.14 | 1.00 | 1.00 | 0.93 |
| *S-CNN SP + Gravity CB* | **0.92** | **0.94** | **0.74** | **0.85** | **2.17** | **0.20** | **0.34** | **2.13** | **0.16** | **3.78** | **4.00** | 0.56 |
| ACLNet | **0.92** | **0.93** | 0.67 | **0.85** | **2.52** | **0.31** | **0.39** | **1.85** | **0.72** | **4.67** | **4.33** | 0.53 |
| DeepVS (OMCNN-2CLSTM) | 0.89 | 0.92 | 0.71 | 0.82 | **2.44** | **0.28** | **0.36** | **2.18** | **0.38** | 5.89 | **5.00** | 0.51 |
| *S-CNN FIX + Gravity CB* | **0.90** | **0.93** | 0.73 | **0.84** | 2.11 | 0.19 | 0.33 | 2.23 | 0.04 | **5.44** | 5.33 | 0.52 |
| *S-CNN SP* | 0.90 | 0.93 | **0.78** | 0.82 | 1.85 | 0.18 | 0.29 | 2.27 | -0.04 | 5.78 | 6.22 | 0.55 |
| *S-CNN FIX* | 0.88 | 0.92 | **0.77** | 0.80 | 1.82 | 0.17 | 0.28 | 2.37 | -0.16 | 7.44 | 7.67 | 0.50 |
| Centre | 0.88 | 0.90 | 0.50 | 0.81 | 1.79 | 0.23 | 0.30 | 2.06 | 0.20 | 10.11 | 9.56 | 0.53 |
| One Human | 0.85 | 0.92 | 0.76 | 0.80 | 3.54 | 0.32 | 0.43 | 7.23 | -6.23 | 11.56 | 11.11 | 0.64 |
| GBVS | 0.83 | 0.88 | 0.61 | 0.76 | 1.33 | 0.18 | 0.22 | 2.38 | -0.22 | 11.44 | 11.56 | 0.54 |
| OBDL-MRF-T | 0.79 | 0.87 | 0.68 | 0.72 | 1.24 | 0.16 | 0.19 | 2.62 | -0.49 | 14.44 | 12.56 | 0.51 |
| OBDL-MRF-TO | 0.79 | 0.87 | 0.69 | 0.72 | 1.23 | 0.15 | 0.18 | 2.64 | -0.51 | 14.67 | 12.56 | 0.52 |
| OBDL-MRF-TC | 0.79 | 0.87 | 0.70 | 0.72 | 1.22 | 0.15 | 0.18 | 2.65 | -0.51 | 14.44 | 12.78 | 0.52 |
| OBDL-MRF-O | 0.79 | 0.87 | 0.69 | 0.72 | 1.20 | 0.16 | 0.18 | 2.67 | -0.52 | 11.67 | 13.67 | 0.51 |
| OBDL-MRF | 0.78 | 0.87 | 0.69 | 0.72 | 1.22 | 0.16 | 0.18 | 2.66 | -0.52 | 12.00 | 13.78 | 0.51 |
| OBDL-MRF-OC | 0.78 | 0.87 | 0.69 | 0.72 | 1.19 | 0.16 | 0.17 | 2.68 | -0.52 | 13.11 | 14.78 | 0.52 |
| OBDL-MRF-C | 0.78 | 0.87 | 0.69 | 0.72 | 1.18 | 0.16 | 0.17 | 2.69 | -0.53 | 14.78 | 15.89 | 0.52 |
| OBDL-T | 0.77 | 0.86 | 0.68 | 0.71 | 1.11 | 0.15 | 0.17 | 2.70 | -0.60 | 17.78 | 17.89 | 0.51 |
| OBDL-S | 0.76 | 0.86 | 0.67 | 0.70 | 1.08 | 0.15 | 0.16 | 2.79 | -0.70 | 18.89 | 19.11 | 0.52 |
| Mathe | 0.73 | 0.86 | 0.67 | 0.69 | 1.28 | 0.17 | 0.17 | 9.45 | -8.48 | 20.44 | 20.67 | 0.51 |
| MSM-SM | 0.75 | 0.85 | 0.66 | 0.70 | 0.91 | 0.15 | 0.13 | 4.01 | -1.96 | 22.00 | 21.67 | **0.59** |
| PMES | 0.72 | 0.83 | 0.66 | 0.67 | 0.88 | 0.14 | 0.13 | 3.18 | -1.24 | 23.11 | 22.00 | **0.58** |
| OBDL | 0.72 | 0.84 | 0.65 | 0.66 | 0.84 | 0.14 | 0.12 | 3.51 | -1.53 | 22.33 | 22.89 | 0.52 |
| AWS-D | 0.70 | 0.84 | 0.64 | 0.65 | 0.73 | 0.13 | 0.11 | 2.89 | -0.95 | 23.00 | 24.00 | 0.44 |
| PIM-ZEN | 0.71 | 0.83 | 0.65 | 0.66 | 0.80 | 0.13 | 0.11 | 3.61 | -1.68 | 24.11 | 24.00 | 0.57 |
| PIM-MCS | 0.70 | 0.83 | 0.65 | 0.65 | 0.69 | 0.13 | 0.10 | 3.82 | -1.91 | 26.22 | 25.78 | 0.54 |
| STSD | 0.69 | 0.83 | 0.62 | 0.65 | 0.46 | 0.12 | 0.07 | 3.44 | -1.68 | 26.33 | 27.44 | 0.53 |
| Permutation | 0.72 | 0.85 | 0.52 | 0.68 | 0.63 | 0.13 | 0.10 | 11.03 | -12.53 | 28.33 | 27.67 | 0.53 |
| PNSP-CS | 0.66 | 0.82 | 0.62 | 0.62 | 0.47 | 0.12 | 0.06 | 3.35 | -1.55 | 28.67 | 28.11 | 0.56 |
| MAM | 0.66 | 0.82 | 0.62 | 0.63 | 0.58 | 0.12 | 0.08 | 5.29 | -4.00 | 29.11 | 28.33 | **0.58** |
| Invariant-K | 0.65 | 0.82 | 0.57 | 0.62 | 0.41 | 0.13 | 0.07 | 5.53 | -4.53 | 29.56 | 30.22 | 0.46 |
| MCSDM | 0.65 | 0.80 | 0.59 | 0.61 | 0.36 | 0.12 | 0.06 | 3.83 | -2.12 | 30.89 | 30.67 | 0.54 |
| Invariant-S | 0.61 | 0.80 | 0.54 | 0.59 | 0.29 | 0.11 | 0.05 | 5.44 | -4.50 | 31.22 | 32.00 | 0.47 |
| Chance | 0.50 | 0.77 | 0.50 | 0.50 | 0.00 | 0.10 | -0.00 | 3.37 | -1.74 | 32.44 | 32.44 | 0.50 |
| Invariant-H | 0.58 | 0.79 | 0.53 | 0.57 | 0.19 | 0.11 | 0.03 | 5.74 | -4.93 | 33.33 | 33.33 | 0.49 |

Table 5. Saliency (fixations) prediction results on Hollywood2, 50-clip subset (fixation samples detected by [4]). Regular averaging was used in all columns with individual metrics, but mean ranks are provided for weighted averaging of statistics as well (marked with $^*$). The rows are sorted by the mean rank for the regular averaging column. Top-3 non-baseline results in each column are **boldified**. In the *Infinite Humans* row, the "inf" value indicates that the sequence, which is analysed in order to get the estimate for this baseline [5], does not seem to converge, at least on the available data.

| Model | AUC-Borji | AUC-Judd | sAUC | accuracy | NSS | SIM | CC | KLD | IG | avg. rank | avg. rank$^*$ |
|---|---|---|---|---|---|---|---|---|---|---|---|
| Infinite Humans | 0.97 | 0.98 | 0.91 | 0.91 | inf | 1.00 | 1.00 | 0.00 | 3.41 | 1.00 | 1.00 |
| ACLNet | **0.91** | **0.92** | 0.68 | **0.84** | **2.50** | **0.39** | **0.47** | **1.40** | **0.52** | **2.89** | **4.22** |
| *S-CNN FIX + Gravity CB* | **0.90** | **0.92** | **0.74** | **0.83** | **2.08** | 0.26 | **0.41** | 1.75 | **-0.12** | **4.56** | **4.11** |
| DeepVS (OMCNN-2CLSTM) | 0.89 | 0.91 | 0.72 | 0.82 | **2.44** | **0.36** | **0.44** | **1.66** | **0.27** | **4.67** | **4.56** |
| *S-CNN SP + Gravity CB* | **0.90** | **0.92** | 0.72 | **0.83** | 1.99 | **0.26** | 0.40 | **1.75** | -0.13 | 5.11 | 5.22 |
| *S-CNN FIX* | 0.88 | 0.90 | **0.78** | 0.80 | 1.84 | 0.24 | 0.36 | 1.88 | -0.31 | 6.67 | 6.67 |
| *S-CNN SP* | 0.87 | 0.90 | **0.76** | 0.79 | 1.72 | 0.24 | 0.34 | 1.89 | -0.33 | 7.56 | 7.44 |
| One Human | 0.87 | 0.92 | 0.75 | 0.82 | 3.21 | 0.37 | 0.48 | 5.45 | -4.46 | 9.78 | 10.00 |
| Centre | 0.85 | 0.88 | 0.51 | 0.78 | 1.64 | 0.29 | 0.34 | 1.72 | -0.14 | 10.33 | 10.56 |
| GBVS | 0.81 | 0.85 | 0.60 | 0.74 | 1.26 | 0.25 | 0.26 | 1.96 | -0.47 | 11.33 | 11.56 |
| OBDL-MRF | 0.77 | 0.84 | 0.68 | 0.71 | 1.28 | 0.23 | 0.25 | 2.20 | -0.75 | 11.33 | 11.78 |
| OBDL-MRF-T | 0.78 | 0.84 | 0.67 | 0.72 | 1.25 | 0.22 | 0.25 | 2.18 | -0.74 | 12.22 | 12.11 |
| OBDL-MRF-O | 0.77 | 0.84 | 0.67 | 0.71 | 1.22 | 0.23 | 0.24 | 2.22 | -0.78 | 13.33 | 13.56 |
| OBDL-MRF-OC | 0.77 | 0.84 | 0.67 | 0.71 | 1.22 | 0.23 | 0.24 | 2.23 | -0.78 | 14.22 | 14.78 |
| OBDL-MRF-TO | 0.77 | 0.84 | 0.67 | 0.71 | 1.25 | 0.22 | 0.24 | 2.21 | -0.77 | 14.33 | 14.22 |
| OBDL-MRF-C | 0.77 | 0.84 | 0.67 | 0.71 | 1.20 | 0.23 | 0.23 | 2.23 | -0.79 | 15.89 | 16.00 |
| OBDL-MRF-TC | 0.77 | 0.84 | 0.67 | 0.71 | 1.21 | 0.22 | 0.23 | 2.22 | -0.80 | 16.78 | 16.22 |
| AWS-D | 0.75 | 0.82 | 0.68 | 0.70 | 1.08 | 0.21 | 0.21 | 2.21 | -0.79 | 18.00 | 17.00 |
| OBDL-T | 0.76 | 0.83 | 0.66 | 0.70 | 1.12 | 0.21 | 0.22 | 2.25 | -0.84 | 18.67 | 18.67 |
| OBDL-S | 0.75 | 0.82 | 0.66 | 0.69 | 1.06 | 0.21 | 0.21 | 2.41 | -1.08 | 20.22 | 20.33 |
| Mathe | 0.73 | 0.82 | 0.67 | 0.69 | 1.27 | 0.22 | 0.22 | 9.11 | -9.23 | 21.67 | 19.44 |
| OBDL | 0.70 | 0.80 | 0.63 | 0.65 | 0.84 | 0.20 | 0.16 | 3.35 | -2.28 | 22.89 | 22.67 |
| Permutation | 0.76 | 0.84 | 0.52 | 0.71 | 1.20 | 0.21 | 0.21 | 7.00 | -7.51 | 23.44 | 25.22 |
| Invariant-K | 0.69 | 0.79 | 0.60 | 0.66 | 0.68 | 0.20 | 0.14 | 5.01 | -4.71 | 25.00 | 24.89 |
| STSD | 0.68 | 0.78 | 0.60 | 0.64 | 0.43 | 0.18 | 0.09 | 2.91 | -1.83 | 25.44 | 26.00 |
| PIM-ZEN | 0.65 | 0.78 | 0.59 | 0.62 | 0.60 | 0.18 | 0.12 | 4.02 | -3.27 | 26.56 | 25.89 |
| PIM-MCS | 0.66 | 0.78 | 0.60 | 0.63 | 0.56 | 0.18 | 0.11 | 4.23 | -3.53 | 26.67 | 26.44 |
| PMES | 0.65 | 0.77 | 0.59 | 0.61 | 0.60 | 0.18 | 0.12 | 3.31 | -2.38 | 27.00 | 26.11 |
| Invariant-S | 0.65 | 0.77 | 0.58 | 0.63 | 0.55 | 0.18 | 0.11 | 4.81 | -4.54 | 27.67 | 27.78 |
| MSM-SM | 0.64 | 0.78 | 0.57 | 0.61 | 0.60 | 0.18 | 0.12 | 6.85 | -7.39 | 28.44 | 29.33 |
| PNSP-CS | 0.61 | 0.75 | 0.56 | 0.58 | 0.25 | 0.15 | 0.05 | 3.17 | -2.26 | 30.11 | 30.56 |
| Invariant-H | 0.62 | 0.75 | 0.55 | 0.60 | 0.39 | 0.17 | 0.08 | 5.01 | -4.83 | 30.89 | 30.89 |
| MCSDM | 0.61 | 0.75 | 0.55 | 0.58 | 0.23 | 0.15 | 0.05 | 3.97 | -3.35 | 31.00 | 31.00 |
| Chance | 0.50 | 0.72 | 0.50 | 0.50 | 0.00 | 0.14 | -0.00 | 2.90 | -1.88 | 31.78 | 31.67 |
| MAM | 0.60 | 0.75 | 0.56 | 0.57 | 0.30 | 0.15 | 0.06 | 6.11 | -6.18 | 32.56 | 32.11 |

Table 6. Saliency (fixation onsets, detection as in [1]) prediction results on Hollywood2, 50-clip subset. Regular averaging was used in all columns with individual metrics, but mean ranks are provided for weighted averaging of statistics as well (marked with *). The rows are sorted by the mean rank for the regular averaging column. Top-3 non-baseline results in each column are **boldified**. In the *Infinite Humans* row, the “inf” value indicates that the sequence, which is analysed in order to get the estimate for this baseline [5], does not seem to converge, at least on the available data.

| Model | AUC-Borji | AUC-Judd | sAUC | accuracy | NSS | SIM | CC | KLD | IG | avg. rank | avg. rank* |
|---|---|---|---|---|---|---|---|---|---|---|---|
| Infinite Humans | 0.97 | 0.98 | 0.85 | 0.90 | inf | 1.00 | 1.00 | 0.00 | 3.03 | 1.00 | 1.00 |
| ACLNet | **0.90** | **0.92** | 0.69 | **0.83** | **2.46** | **0.40** | **0.48** | **1.40** | **0.43** | **3.44** | **4.22** |
| *S-CNN FIX + Gravity CB* | **0.90** | **0.92** | **0.75** | **0.83** | **2.10** | 0.26 | **0.42** | 1.70 | **-0.14** | **4.11** | **3.89** |
| DeepVS (OMCNN-2CLSTM) | 0.88 | 0.91 | 0.71 | 0.81 | **2.32** | **0.37** | **0.44** | **1.69** | **0.13** | **4.67** | **5.00** |
| *S-CNN SP + Gravity CB* | **0.90** | **0.92** | 0.73 | **0.83** | 2.01 | **0.27** | 0.42 | **1.69** | -0.16 | 5.00 | **5.00** |
| *S-CNN FIX* | 0.88 | 0.90 | **0.79** | 0.80 | 1.86 | 0.24 | 0.37 | 1.84 | -0.34 | 6.78 | 6.44 |
| *S-CNN SP* | 0.87 | 0.90 | **0.77** | 0.79 | 1.74 | 0.25 | 0.36 | 1.83 | -0.36 | 7.44 | 7.44 |
| Centre | 0.85 | 0.88 | 0.51 | 0.78 | 1.65 | 0.30 | 0.36 | 1.66 | -0.16 | 10.11 | 10.22 |
| One Human | 0.85 | 0.91 | 0.74 | 0.80 | 3.24 | 0.37 | 0.50 | 5.96 | -5.29 | 10.56 | 10.89 |
| GBVS | 0.82 | 0.86 | 0.61 | 0.75 | 1.31 | 0.26 | 0.27 | 1.89 | -0.47 | 11.11 | 11.44 |
| OBDL-MRF-O | 0.78 | 0.84 | 0.68 | 0.72 | 1.27 | 0.23 | 0.24 | 2.19 | -0.74 | 11.78 | 12.78 |
| OBDL-MRF | 0.78 | 0.84 | 0.68 | 0.72 | 1.29 | 0.23 | 0.25 | 2.17 | -0.75 | 12.78 | 12.44 |
| OBDL-MRF-OC | 0.78 | 0.84 | 0.68 | 0.72 | 1.27 | 0.23 | 0.24 | 2.19 | -0.75 | 12.89 | 14.00 |
| OBDL-MRF-C | 0.78 | 0.84 | 0.68 | 0.72 | 1.25 | 0.23 | 0.24 | 2.20 | -0.76 | 14.22 | 15.67 |
| OBDL-MRF-T | 0.78 | 0.84 | 0.67 | 0.72 | 1.24 | 0.23 | 0.25 | 2.16 | -0.77 | 15.11 | 12.78 |
| OBDL-MRF-TO | 0.78 | 0.84 | 0.68 | 0.71 | 1.24 | 0.22 | 0.24 | 2.18 | -0.79 | 15.22 | 15.33 |
| OBDL-MRF-TC | 0.77 | 0.84 | 0.68 | 0.71 | 1.22 | 0.22 | 0.24 | 2.19 | -0.80 | 17.11 | 16.11 |
| AWS-D | 0.76 | 0.83 | 0.69 | 0.70 | 1.09 | 0.21 | 0.21 | 2.15 | -0.80 | 18.22 | 17.67 |
| OBDL-T | 0.77 | 0.84 | 0.67 | 0.71 | 1.18 | 0.22 | 0.23 | 2.21 | -0.83 | 18.56 | 18.56 |
| OBDL-S | 0.76 | 0.83 | 0.67 | 0.70 | 1.14 | 0.22 | 0.22 | 2.37 | -1.05 | 19.89 | 19.89 |
| Mathe | 0.73 | 0.83 | 0.67 | 0.69 | 1.33 | 0.23 | 0.23 | 9.12 | -9.00 | 21.89 | 20.44 |
| Permutation | 0.75 | 0.84 | 0.52 | 0.71 | 1.45 | 0.22 | 0.24 | 7.13 | -7.77 | 22.33 | 23.56 |
| OBDL | 0.72 | 0.81 | 0.64 | 0.67 | 0.90 | 0.20 | 0.17 | 3.31 | -2.13 | 22.78 | 22.67 |
| Invariant-K | 0.70 | 0.79 | 0.60 | 0.66 | 0.74 | 0.20 | 0.16 | 4.75 | -4.48 | 25.00 | 25.56 |
| STSD | 0.69 | 0.79 | 0.61 | 0.65 | 0.46 | 0.18 | 0.10 | 2.81 | -1.75 | 25.11 | 25.44 |
| PIM-ZEN | 0.65 | 0.77 | 0.60 | 0.61 | 0.60 | 0.18 | 0.13 | 3.96 | -4.02 | 27.11 | 27.00 |
| Invariant-S | 0.66 | 0.78 | 0.58 | 0.63 | 0.59 | 0.19 | 0.13 | 4.58 | -4.33 | 27.22 | 28.11 |
| MSM-SM | 0.66 | 0.79 | 0.59 | 0.63 | 0.70 | 0.19 | 0.13 | 6.31 | -6.61 | 27.22 | 27.00 |
| PIM-MCS | 0.65 | 0.78 | 0.60 | 0.62 | 0.56 | 0.18 | 0.12 | 4.16 | -4.31 | 27.22 | 26.78 |
| PMES | 0.64 | 0.77 | 0.59 | 0.61 | 0.59 | 0.18 | 0.13 | 3.28 | -3.36 | 27.44 | 26.33 |
| PNSP-CS | 0.59 | 0.75 | 0.56 | 0.58 | 0.25 | 0.15 | 0.06 | 3.12 | -3.23 | 30.11 | 30.00 |
| Invariant-H | 0.63 | 0.76 | 0.55 | 0.61 | 0.45 | 0.17 | 0.09 | 4.76 | -4.56 | 30.89 | 30.89 |
| MCSDM | 0.59 | 0.74 | 0.55 | 0.57 | 0.21 | 0.16 | 0.05 | 3.92 | -4.32 | 31.56 | 31.44 |
| Chance | 0.50 | 0.72 | 0.50 | 0.50 | 0.01 | 0.14 | -0.00 | 2.84 | -1.92 | 31.89 | 31.67 |
| MAM | 0.59 | 0.74 | 0.56 | 0.57 | 0.30 | 0.16 | 0.07 | 5.96 | -6.77 | 32.22 | 32.33 |

Table 7. Saliency (fixation onsets, provided with the data set [3]) prediction results on CITIUS-R. Regular averaging was used in all columns with individual metrics, but mean ranks are provided for weighted averaging of statistics as well (marked with *). The rows are sorted by the mean rank for the regular averaging column. Top-3 non-baseline results in each column are **boldified**.

| Model | AUC-Borji | AUC-Judd | sAUC | accuracy | NSS | SIM | CC | KLD | IG | avg. rank | avg. rank* |
|---|---|---|---|---|---|---|---|---|---|---|---|
| *S-CNN SP + Gravity CB* | **0.87** | **0.87** | 0.71 | **0.80** | **1.78** | **0.41** | **0.52** | **1.13** | **0.28** | **3.33** | **3.33** |
| ACLNet | **0.87** | **0.87** | 0.70 | **0.80** | **2.03** | **0.47** | **0.53** | 1.28 | **0.33** | **3.33** | **3.44** |
| *S-CNN FIX + Gravity CB* | **0.87** | **0.87** | 0.71 | **0.79** | **1.81** | 0.40 | **0.52** | **1.16** | **0.24** | **3.89** | **4.00** |
| *S-CNN SP* | 0.85 | 0.85 | 0.74 | 0.78 | 1.56 | 0.38 | 0.45 | **1.24** | 0.11 | 4.78 | 4.22 |
| *S-CNN FIX* | 0.84 | 0.84 | **0.74** | 0.77 | 1.54 | 0.36 | 0.43 | 1.29 | 0.04 | 5.56 | 5.33 |
| AWS-D | 0.79 | 0.79 | **0.77** | 0.73 | 1.72 | 0.34 | 0.41 | 1.46 | 0.00 | 7.22 | 7.00 |
| GBVS | 0.83 | 0.83 | 0.67 | 0.76 | 1.58 | 0.37 | 0.40 | 1.33 | 0.13 | 7.56 | 8.00 |
| DeepVS (OMCNN-2CLSTM) | 0.81 | 0.81 | 0.64 | 0.75 | 1.66 | **0.41** | 0.44 | 1.66 | -0.31 | 8.22 | 8.11 |
| OBDL-MRF-O | 0.79 | 0.79 | **0.74** | 0.73 | 1.48 | 0.34 | 0.37 | 2.28 | -1.12 | 9.89 | 10.22 |
| Centre | 0.81 | 0.81 | 0.51 | 0.75 | 1.30 | 0.39 | 0.40 | 1.31 | 0.00 | 10.56 | 11.00 |
| OBDL-T | 0.78 | 0.78 | 0.74 | 0.72 | 1.44 | 0.33 | 0.35 | 2.21 | -1.05 | 11.11 | 11.33 |
| OBDL-MRF-OC | 0.78 | 0.78 | 0.74 | 0.72 | 1.46 | 0.33 | 0.36 | 2.30 | -1.15 | 11.22 | 11.56 |
| OBDL-MRF-C | 0.78 | 0.78 | 0.74 | 0.72 | 1.43 | 0.33 | 0.35 | 2.31 | -1.16 | 13.11 | 13.22 |
| OBDL-MRF-TO | 0.77 | 0.77 | 0.72 | 0.71 | 1.38 | 0.33 | 0.35 | 2.25 | -1.14 | 13.33 | 13.56 |
| OBDL-MRF | 0.78 | 0.78 | 0.73 | 0.72 | 1.40 | 0.33 | 0.35 | 2.28 | -1.15 | 13.67 | 13.67 |
| OBDL-MRF-T | 0.77 | 0.77 | 0.71 | 0.71 | 1.29 | 0.33 | 0.33 | 2.24 | -1.14 | 15.33 | 15.22 |
| OBDL-MRF-TC | 0.77 | 0.77 | 0.72 | 0.71 | 1.32 | 0.32 | 0.33 | 2.27 | -1.17 | 15.56 | 15.33 |
| OBDL-S | 0.76 | 0.76 | 0.72 | 0.71 | 1.34 | 0.32 | 0.33 | 2.98 | -2.07 | 17.33 | 17.44 |
| STSD | 0.75 | 0.75 | 0.71 | 0.70 | 1.16 | 0.30 | 0.26 | 2.43 | -1.07 | 18.00 | 17.33 |
| OBDL | 0.72 | 0.73 | 0.69 | 0.67 | 1.18 | 0.28 | 0.27 | 4.31 | -3.58 | 20.78 | 21.78 |
| Invariant-K | 0.72 | 0.72 | 0.66 | 0.69 | 0.98 | 0.31 | 0.27 | 4.12 | -3.97 | 20.78 | 20.33 |
| Invariant-S | 0.69 | 0.69 | 0.63 | 0.67 | 0.76 | 0.28 | 0.21 | 4.18 | -4.04 | 22.78 | 22.33 |
| Permutation | 0.73 | 0.73 | 0.51 | 0.68 | 0.67 | 0.26 | 0.20 | 5.10 | -5.28 | 24.78 | 24.44 |
| MSM-SM | 0.68 | 0.69 | 0.63 | 0.64 | 0.91 | 0.25 | 0.21 | 6.45 | -6.65 | 25.44 | 25.56 |
| Invariant-H | 0.66 | 0.66 | 0.59 | 0.64 | 0.55 | 0.26 | 0.16 | 4.36 | -4.29 | 25.78 | 25.44 |
| PIM-MCS | 0.65 | 0.65 | 0.63 | 0.62 | 0.71 | 0.26 | 0.17 | 5.10 | -5.36 | 26.22 | 26.33 |
| PIM-ZEN | 0.64 | 0.64 | 0.61 | 0.60 | 0.73 | 0.26 | 0.17 | 5.22 | -5.49 | 26.78 | 26.67 |
| PMES | 0.62 | 0.62 | 0.59 | 0.58 | 0.63 | 0.27 | 0.18 | 4.54 | -4.67 | 27.00 | 26.89 |
| PNSP-CS | 0.62 | 0.62 | 0.61 | 0.59 | 0.51 | 0.24 | 0.12 | 3.14 | -3.10 | 27.22 | 27.44 |
| MCSDM | 0.63 | 0.63 | 0.61 | 0.60 | 0.51 | 0.24 | 0.13 | 4.96 | -5.43 | 28.11 | 28.33 |
| Chance | 0.50 | 0.50 | 0.50 | 0.50 | -0.00 | 0.22 | 0.00 | 2.25 | -1.42 | 28.22 | 28.00 |
| MAM | 0.56 | 0.56 | 0.54 | 0.54 | 0.33 | 0.21 | 0.09 | 8.20 | -9.66 | 31.11 | 31.11 |
